# Supplementary material for: EVEREST: Efficient Masked Video Autoencoder by Removing Redundant Spatiotemporal Tokens
Source: arXiv:2211.10636 source file (2024-06-20)
Supplement: Supplementary file 1 [file supplement_table_ablation_sampling.tex]

\begin{wraptable}{r}{3.cm}
\centering
% \vspace{-0.1in}
%\addtolength{\tabcolsep}{-2.8pt}  
\caption{\small \bf Ablation study of motion-aware adaptive frame selection of MATS. }
\vspace{0.1in}
\resizebox{0.18\textwidth}{!}{

\begin{tabular}{c c}
        \toprule
        \vspace{-0.02in}
        $\alpha$ & \textbf{Acc. (\%)} \\
        \midrule
        { -} & { 73.17}\\
        { 1.3} & { 73.54}\\
        \highlight{ 1.5} & { \textbf{73.85}}\\
        { 1.8} & { 73.79}\\
        { 2.0} & { 73.80}\\
\bottomrule
\end{tabular}}
\label{tab:ablation_sampling}
\end{wraptable}
