# Supplementary material for: EVEREST: Efficient Masked Video Autoencoder by Removing Redundant Spatiotemporal Tokens
Source: arXiv:2211.10636 source file (2024-06-20)
Supplement: Supplementary file 2 [file supplement_table_hyperparams_oscc.tex]

\begin{table}[h]
\vspace{-0.15in}
\begin{minipage}{0.49\linewidth}
    \vspace{-0.1in}
    \vspace{0.05in}
\centering
        \resizebox{1.0\textwidth}{!}{

\begin{tabular}{c|c}
& {OSCC}\\
\midrule
optimizer&\\
base learning rate&\\
weight decay&\\
batch size&\\
\bottomrule
\end{tabular}}
\end{minipage}
\hfill
\begin{minipage}{0.49\linewidth}
    \vspace{-0.1in}
    \vspace{0.05in}
\centering
        \resizebox{1.0\textwidth}{!}{

\begin{tabular}{c|c}
& {OSCC}\\
\midrule
optimizer&\\
base learning rate&\\
weight decay&\\
batch size&\\
\bottomrule
\end{tabular}}
\end{minipage}
    \vspace{-0.05in}
    \caption{\small \textbf{Pre-training (Left) and Fine-tuning (Right) settings for OSCC.}}
    \label{tab:supplement_table_hyperparams_oscc}
    \vspace{-0.1in}
\end{table}
