# Supplementary material for: EVEREST: Efficient Masked Video Autoencoder by Removing Redundant Spatiotemporal Tokens
Source: arXiv:2211.10636 source file (2024-06-20)
Supplement: Supplementary file 3 [file supplement_table_hyperparams_oscc_ft.tex]

\vspace{0.05in}
\centering
        \resizebox{1.0\textwidth}{!}{

\begin{tabular}{c|c}
& {OSCC}\\
\midrule
optimizer&\\
base learning rate&\\
weight decay&\\
batch size&\\
\bottomrule
\end{tabular}}
